# Supplementary material for: REAL: Resolving Knowledge Conflicts in Knowledge-Intensive Visual Question Answering via Reasoning-Pivot Alignment
Source: arXiv:2602.14065 source file (2026-05-30)
Supplement: Supplementary file 1 [file case_study_appendix_1.pdf]

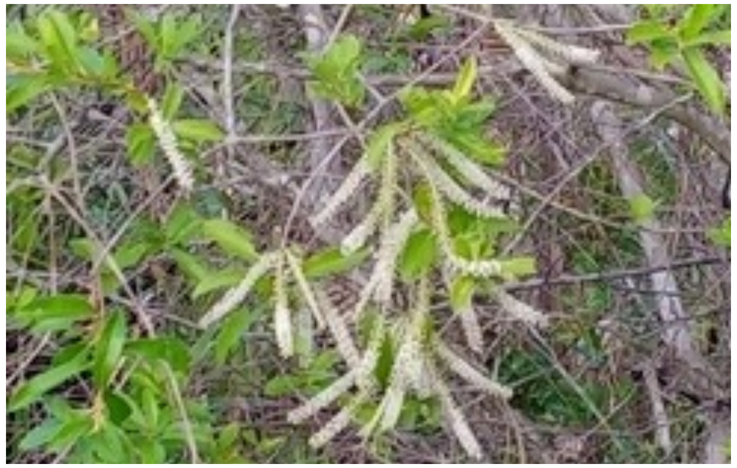

**Q: Who did this plant's native country join fighting against?**

| Greedy: | VCD: |
| --- | --- |
| *United Nations* ✗ | *United Nations* ✗ |
| **CAD:** | **RPGD(Ours):** |
| *United Nations* ✗ | *Axis powers* ✓ |

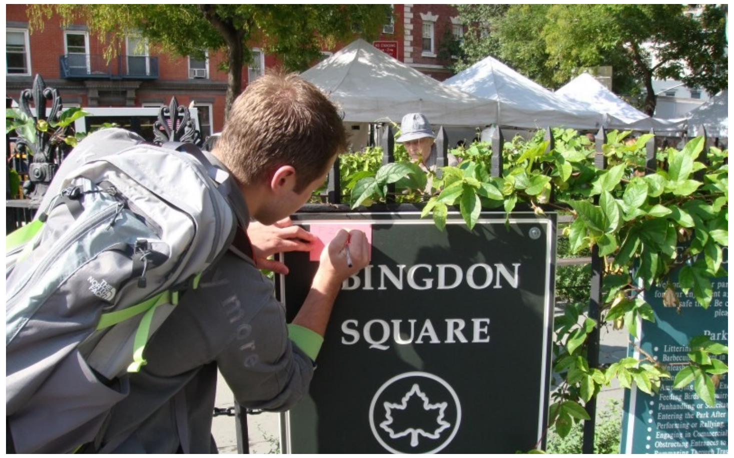


**Q: What street borders this park?**

| Greedy: | VCD: |
| --- | --- |
| *Duane Street* ✗ | *Duane Street* ✗ |
| **CAD:** | **RPGD(Ours):** |
| *Duane Street* ✗ | *Bank Street* ✓ |

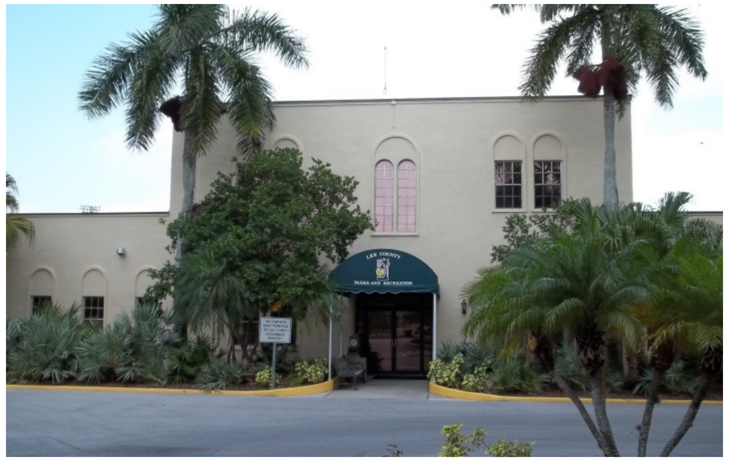

**Q: When was the land for this ballpark donated?**

| Greedy: | VCD: |
| --- | --- |
| *1951* ✗ | *1951* ✗ |
| **CAD:** | **RPGD(Ours):** |
| *1951* ✗ | *1920* ✓ |

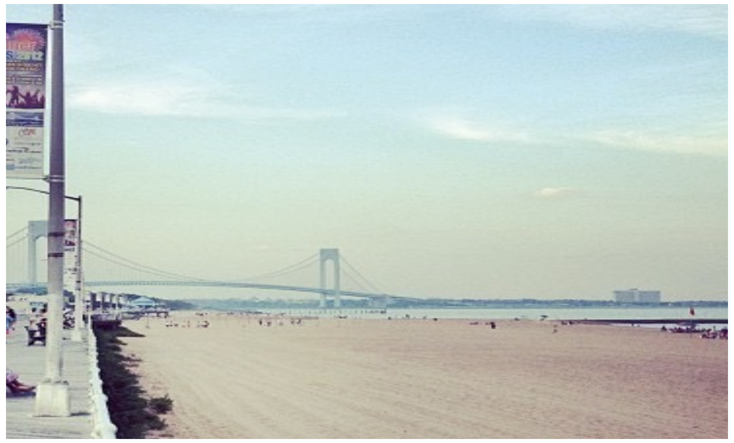

**Q: What borough is connected to New Jersey via this bridge?**

| Greedy: | VCD: |
| --- | --- |
| *Staten Island* ✗ | *Staten Island* ✗ |
| **CAD:** | **RPGD(Ours):** |
| *Staten Island* ✗ | *Long Island* ✓ |

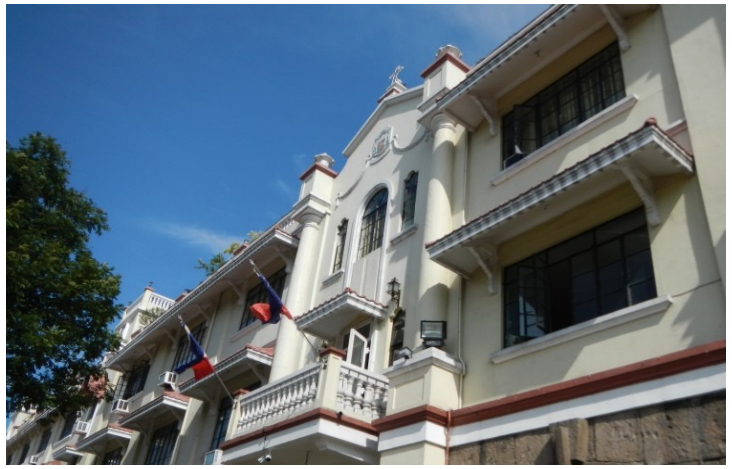

**Q: When was the baptistry of this cathedral consecrated?**

| Greedy: | VCD: |
| --- | --- |
| *June* ✗ | *June* ✗ |
| **CAD:** | **RPGD(Ours):** |
| *February* ✓ | *February* ✓ |

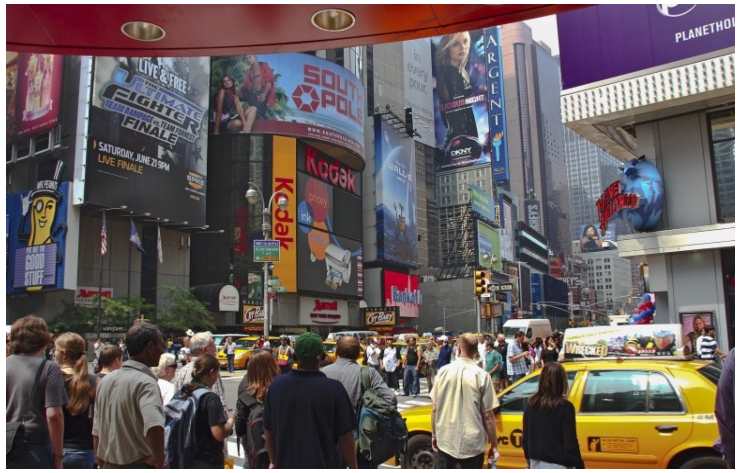


**Q: How many floors are there in this building?**

| Greedy: | VCD: |
| --- | --- |
| *50* ✗ | *50* ✗ |
| **CAD:** | **RPGD(Ours):** |
| *51* ✓ | *51* ✓ |

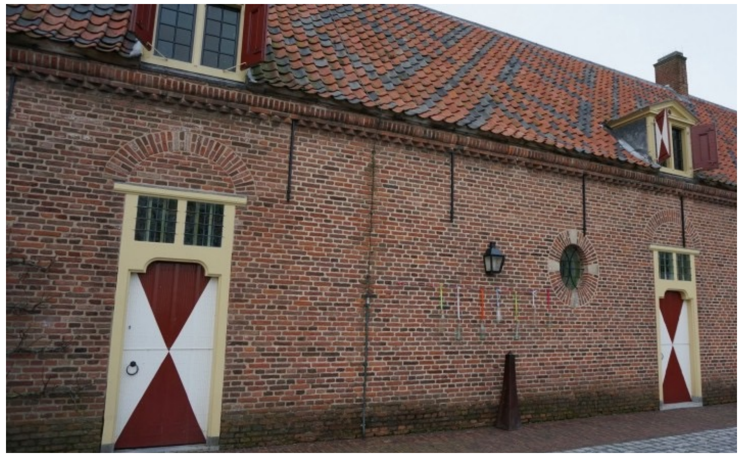

**Q: What material was found during this castle's restoration?**

| Greedy: | VCD: |
| --- | --- |
| *Loam* ✗ | *Loam* ✗ |
| **CAD:** | **RPGD(Ours):** |
| *Loam* ✗ | *Silver&Bronze* ✓ |

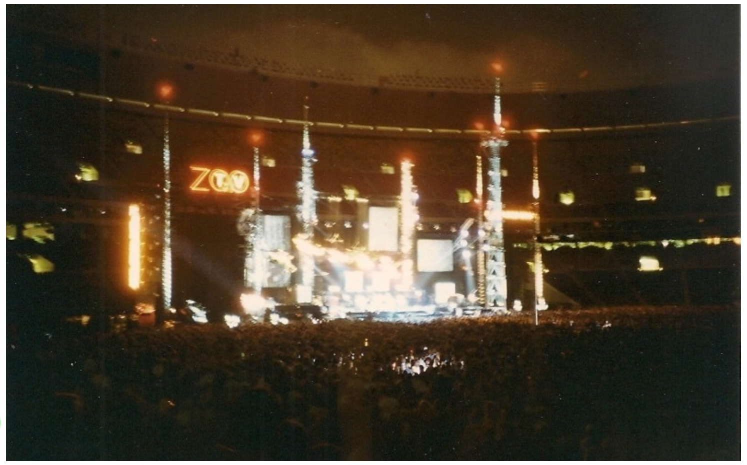


**Q: How many people can this stadium host?**

| Greedy: | VCD: |
| --- | --- |
| *66,000* ✗ | *65.358* ✓ |
| **CAD:** | **RPGD(Ours):** |
| *65,358* ✓ | *65.358* ✓ |

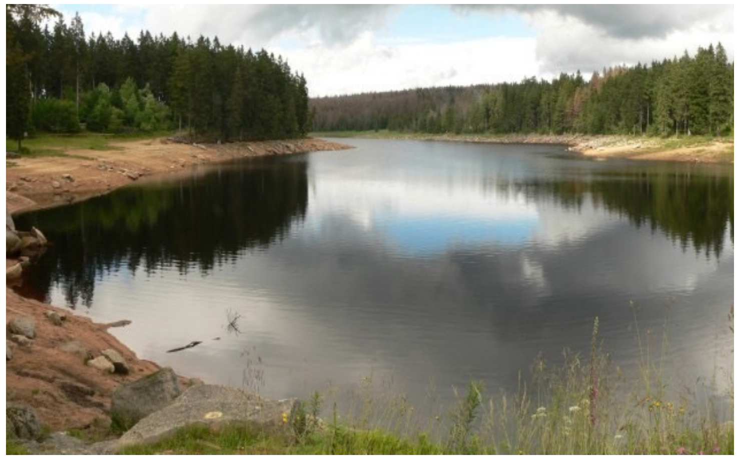

**Q: In which country is this reservoir located?** *Germany* ✓

| Greedy: | VCD: |
| --- | --- |
| *Sweden* ✗ | *Sweden* ✗ |
| **CAD:** | **RPGD(Ours):** |
| *Sweden* ✗ | *Sweden* ✗ |

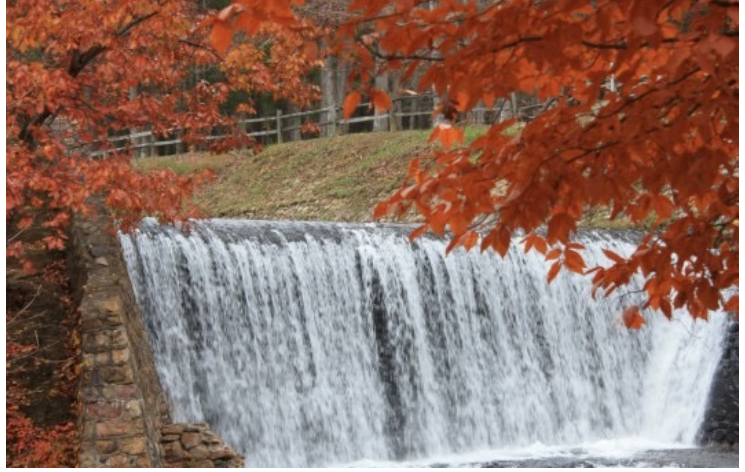

**Q: In which decade did this park's dam receive that award?**

| Greedy: | VCD: |
| --- | --- |
| *1930s* ✗ | *1990s* ✓ |
| **CAD:** | **RPGD(Ours):** |
| *1990s* ✓ | *1930s* ✗ |

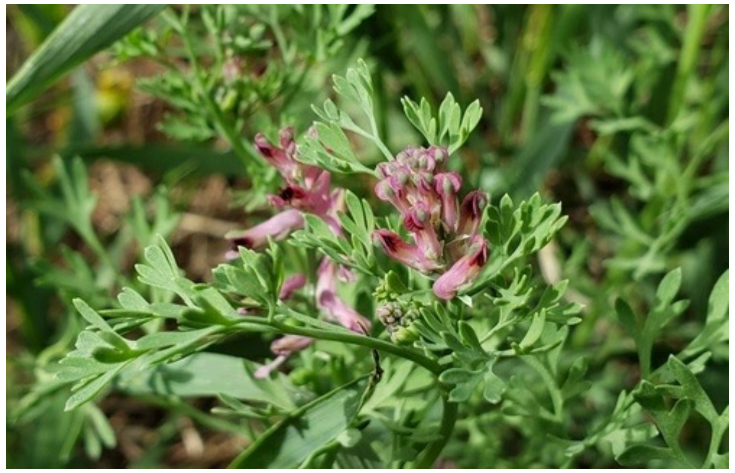

**Q: In what country can you find this plant?** *Serbia* ✓

| Greedy: | VCD: |
| --- | --- |
| *Ukraine* ✗ | *Ukraine* ✗ |
| **CAD:** | **RPGD(Ours):** |
| *Ukraine* ✗ | *Ukraine* ✗ |

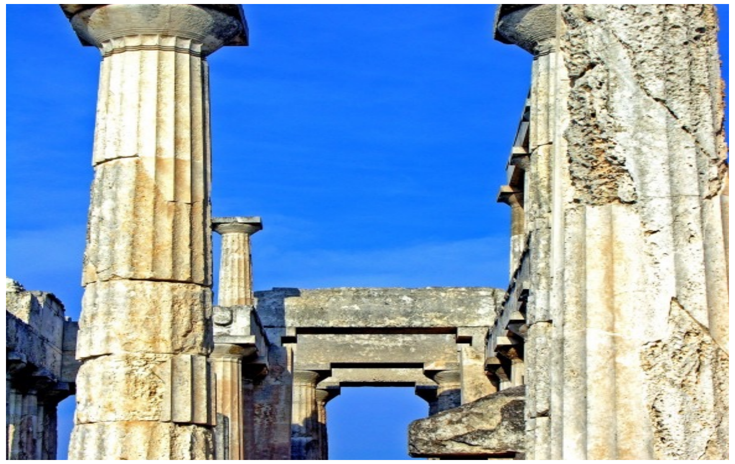

**Q: Where was this temple located on paros?** *Delion* ✓

| Greedy: | VCD: |
| --- | --- |
| *Valencia* ✗ | *Metapontum* ✗ |
| **CAD:** | **RPGD(Ours):** |
| *Paros* ✗ | *Paros* ✗ |

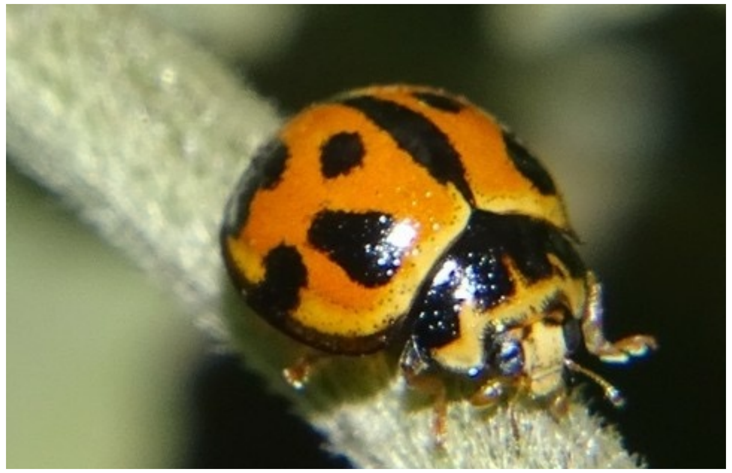

**Q: In which country does this insect live?** *Australia* ✓

| Greedy: | VCD: |
| --- | --- |
| *United States* ✗ | *United States* ✗ |
| **CAD:** | **RPGD(Ours):** |
| *United States* ✗ | *United States* ✗ |

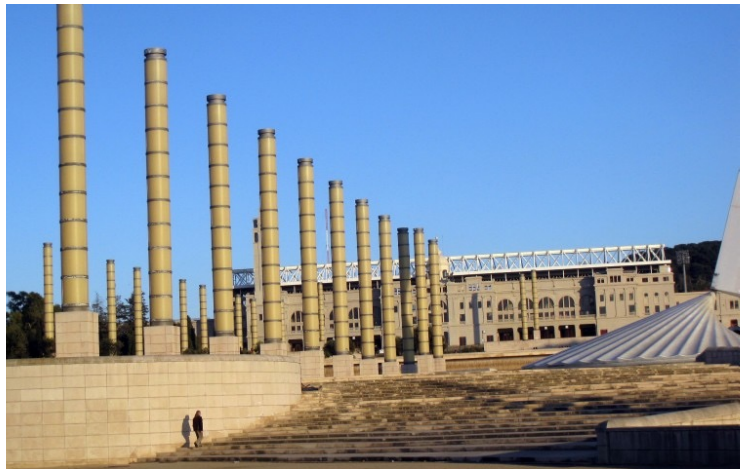

**Q: How many square kilometers is this park?** 18 ✓

| Greedy: | VCD: |
| --- | --- |
| *20* ✗ | *20* ✗ |
| **CAD:** | **RPGD(Ours):** |
| *20* ✗ | *20* ✗ |

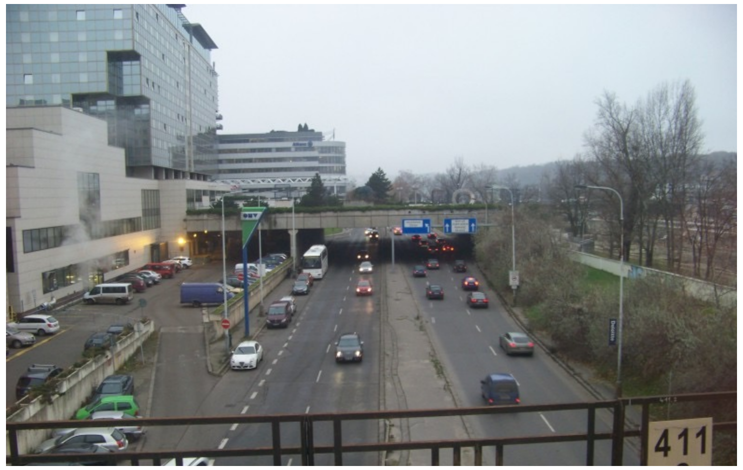


**Q: What city is this hotel located in?** *Prague* ✓

| Greedy: | VCD: |
| --- | --- |
| *Würzburg* ✗ | *Würzburg* ✗ |
| **CAD:** | **RPGD(Ours):** |
| *Würzburg* ✗ | *Würzburg* ✗ |

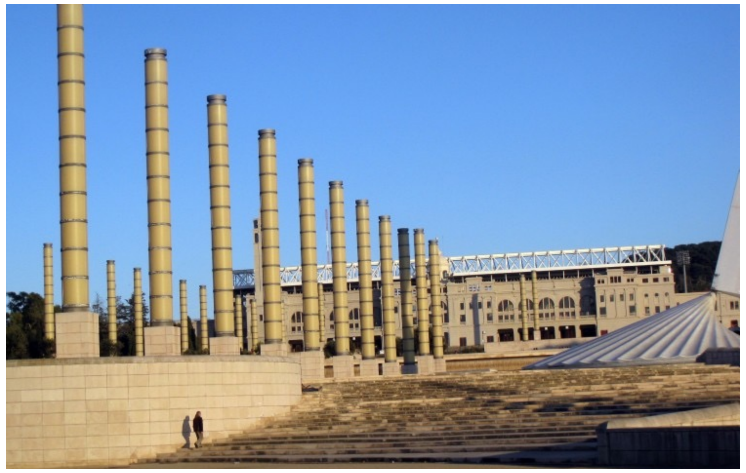

**Q: What type of columns divide the facade of this cathedral?**

| Greedy: | VCD: |
| --- | --- |
| *pilasters* ✗ | *pilasters* ✗ |
| **CAD:** | **RPGD(Ours):** |
| *Doric* ✓ | *pilasters* ✗ |
